# Supplementary material for: Untidy Data: The Unreasonable Effectiveness of Tables
Source: arXiv:2106.15005 source file (2021-06-28)
Supplement: Supplementary file 1 [file appendix.tex]

\section{Appendix}
This supplemental material contains the following:

\subsection{Study materials}

Participants were recruited through userinterviews.com and by targeted email.

\begin{enumerate}
    \item \textbf{Study description for participant.pdf}: Recruitment description of study.
    \item \textbf{Study confidentiality.pdf}: Data Confidentiality 
    \item \textbf{ScreenerSurvey.pdf}: Survey used to screen participants. Note that applicants were not considered eligible if they answered affirmatively to the options marked in red.
    \item \textbf{Study script.pdf}: The script used by our experimenter as the basis for conducting the semi-structured interviews.
\end{enumerate}

\subsection{Results}
\begin{itemize}
    \item \textbf{Sketches}: 
A folder of sketches from 8 of the 12 participants are provided in response to our prompting for them to draw ``the main components and relationships in [their] data.'' The remaining participants generated sketches but did not give permission due to concerns about data confidentiality. In the filenames of the sketches ``P[number]Sketch.jpg'', P[number] corresponds to the same participant ID as in Table 1 in the main paper. ``SampleSketch.jpg'' denotes the sample sketch (based on a fictional dataset about movies) we used as instruction for the participants. 
\end{itemize}

We are unable to provide screenshots or source data schema used by our participants as in all cases this was proprietary and confidential. Participants were unwilling to share details of their organizational data with people other than the three study researchers.

In the main body of the paper we include representative quotations and demographic information about our participants. However, as per our study protocol and consent form, and to avoid breaches of confidentiality or anonymity, we do not include the full video or transcripts of our interviews from these sessions.

\section{Additional Discussion}

\subsection{Data Sketches}

Prior to the central task, we asked for our participants to draw their data model, elicited as ``can you briefly draw on a sheet of paper what you think the main components and relationships in the data should be related to what you want to find out?'' In our initial study planning, we were broadly interested in how participants conceptualized and manipulated their data. Our solicitation of sketches of the participants' data models was originally conducted with that aim in mind, to afford us the capability to analyze how the participant's imagined structure reflected the reality of their data work. However, as the focus of our investigation shifted to tables, these sketches were less central to our research question and so we did not conduct any thorough content analysis on them. We still believe that the elicitation task had benefits in that it encouraged the participants to pause and reflect on the data they generated for us. 

Nonetheless, some patterns emerge fro m a cursory analysis. For instance, while our sample sketch we used for solicitation was meant to represent a snowflake-style schema showing interactions of different tables in a fictional database of movie information, our participants largely did not draw relations between multiple tables, but other aspects of their understanding of the data. For instance, both P3 and P7 drew flow charts showing their work process (for instance, the combination of data from Shopify and Google Analytics for P3, and move from Tableau Prep to Tableau Desktop and so on for P7). P1 and P8, by contrast, drew taxonomies of the different sorts of entities and stakeholders represented in their dataset. A conjecture that awaits more information is that the deep formal models of data that are expected by certain software (for instance, to perform joins in software by Tableau) are poor matches for the rich mental models data workers form over long exposure to and experience with their data.

\subsection{Tidy versus Untidy Tables}
We more explicitly compare the Wickham~\cite{wickham_tidy_2014} notion of ``tidy'' data with our notion of ``rich'' or ``untidy'' tables here (see \autoref{fig:tidyversus}). 

\begin{figure}[h]
     \centering
     \begin{subfigure}[b]{\columnwidth}
         \centering
         \includegraphics[width=\textwidth]{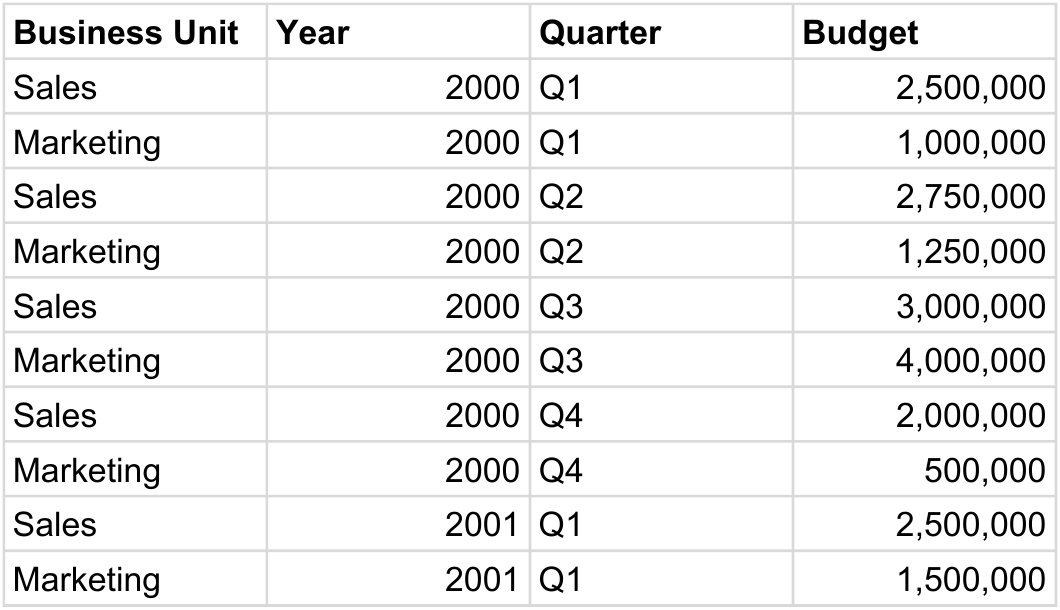}
         \caption{A ``tidy'' table.}
         \label{fig:tidy}
     \end{subfigure}
     
     \begin{subfigure}[b]{\columnwidth}
         \centering
         \includegraphics[width=\textwidth]{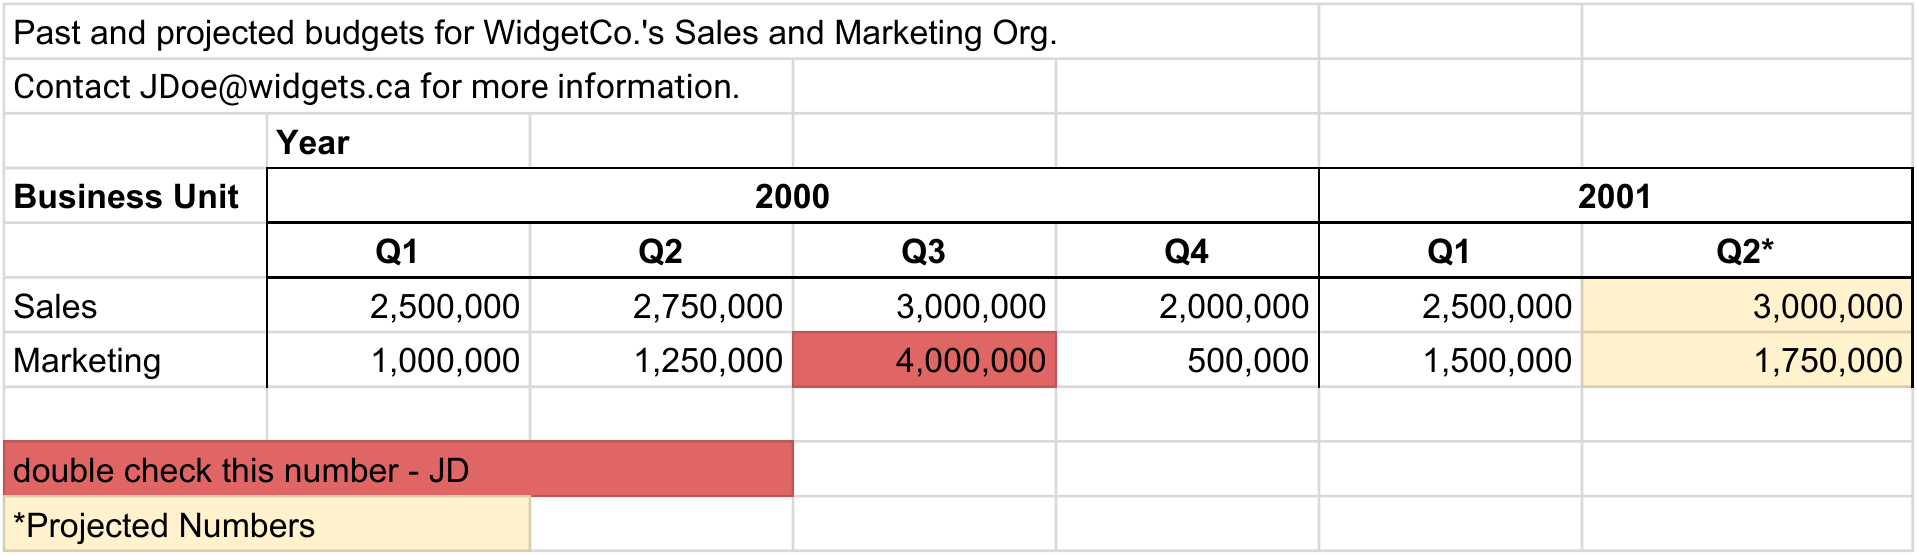}
         \caption{A potential ``rich'' or ``untidy'' table of the same data.}
         \label{fig:untidy}
     \end{subfigure}
        \caption{A juxtaposition of potential ``tidy'' and ``untidy'' views of the same data.}
        \label{fig:tidyversus}
\end{figure}

In a ``tidy'' table, each observation is a row, and each column is a variable, resulting in a ``tall'' format. This format has many benefits for analysis and reshaping. A ``rich'' (or ``untidy'') table, by contrast, has many structures that are useful for human legibility and learning (such as annotations, multi-column structures, and a ``wide'' format), but many of these structures are lost or very difficult to recreate when exported to other tools. (We note that how to automate the parsing of these structures into analytically-ready tidy tables while retaining some of the rich semantics is an area of active research \cite{chen2014integrating}, but discussion of these methods in detail is beyond the scope of this paper. )

As a working example, a ``tidy'' sheet as in \autoref{fig:tidy} is ``tall''. It has one header row and ten rows of data (versus two rows of header information and two rows of data for the ``untidy'' version) and could be directly exported as a csv and then imported into standard charting tools for visualization. \autoref{fig:untidy} is ``wide'' (with six data columns). It would likely require additional parsing and reshaping steps (say, through mixed-initiative systems~\cite{chen2014integrating,hoffswell_augmenting_2018}) to be ready for use in another system. Yet, \autoref{fig:untidy} is arguably more human readable: for instance, it is easier to tell at a glance whether budgets for a particular department are going up or down over time. This legibility is further increased by additional human-generated aides for understanding, such as titles and captions, visual or textual structure (e.g., using multi-cell structures to set apart each year of data), and the ability to ``mark up'' the table with caveats, oddities, or action items.
