# Supplementary material for: Untidy Data: The Unreasonable Effectiveness of Tables
Source: arXiv:2106.15005 ancillary file (2021-06-28)
Supplement: Supplementary file 3 [file Study_script.pdf]

### Study materials:

- Laptop
- Zoom to record screen and audio
- Pen and Blank White Paper

| Script                                                                                                                                                                                                                                                                                                                                                                                                                                                                                                                                                                                                                                                                                                                                                                                                                                                                                                                                                                                                                                                                                                                                                                                                                            | Actions                                                                                                                                                                                                                                                                                               | Sessions Phase         |
|-----------------------------------------------------------------------------------------------------------------------------------------------------------------------------------------------------------------------------------------------------------------------------------------------------------------------------------------------------------------------------------------------------------------------------------------------------------------------------------------------------------------------------------------------------------------------------------------------------------------------------------------------------------------------------------------------------------------------------------------------------------------------------------------------------------------------------------------------------------------------------------------------------------------------------------------------------------------------------------------------------------------------------------------------------------------------------------------------------------------------------------------------------------------------------------------------------------------------------------|-------------------------------------------------------------------------------------------------------------------------------------------------------------------------------------------------------------------------------------------------------------------------------------------------------|------------------------|
| <p>Hi, thanks for taking the time to participate in our study today. My name is [Experimenter Name] and I will be guiding you through this session.</p> <p>The goal of our study today is to better understand how people think about, manipulate and work with their data.</p> <p>In the study we would like you to tell us about your data (that you brought with you today) and how you go about making sense of/answering your questions/learning about it (what you can do with it) and/or communicating it to others (if applicable). We're interested in how you understand the the kind of data you work with, how you manipulate this data, and what steps you currently use to understand relationships in your data.</p>                                                                                                                                                                                                                                                                                                                                                                                                                                                                                               | <p><i>Moderators:</i></p> <p>- Initialize screen recording</p> <p><i>Notetakers:</i></p> <p>- Load notetaking form. Note name and date.</p>                                                                                                                                                           | Introduction           |
| <p>Before we proceed with the study, I want to let you know about how we collect and use data.</p> <p>There are three ways that we collect data for this session.</p> <ul style="list-style-type: none"><li>● First, we will record audio and screen captures for this session.</li><li>● Second, a notetaker will be taking notes of our session.</li><li>● Third, you may optionally provide us with images, data dictionaries, data samples, or schema of the data you work with.</li></ul> <p>All data will be securely stored and only the study leaders will have access to the raw data.</p> <p>All of this data will be analyzed at the end of the study and we will only share the anonymized results internally with our development teams at Tableau or in publication. If we do publicly release any results of the study, they will be anonymized. There's one particular exception to this: if we would like to use an image that you have provided us in a publication, we will get explicit written ermission from you. At any point in the study, you can decide that you don't want to continue anymore. So knowing how we're going to be using your data for this analysis, do you still want to continue?</p> | <p><i>Moderators:</i></p> <p>- Obtain consent for study participation.</p> <p><b>Trouble Shooting:</b></p> <p>If participant has issues with data collection, ask them if there is some level of data collection they do consent to.</p> <p>At a minimum, participant must consent to notetaking.</p> |                        |
|                                                                                                                                                                                                                                                                                                                                                                                                                                                                                                                                                                                                                                                                                                                                                                                                                                                                                                                                                                                                                                                                                                                                                                                                                                   |                                                                                                                                                                                                                                                                                                       |                        |
| 1. How do you use data in your job?                                                                                                                                                                                                                                                                                                                                                                                                                                                                                                                                                                                                                                                                                                                                                                                                                                                                                                                                                                                                                                                                                                                                                                                               | probe for what they consider as different types of data:                                                                                                                                                                                                                                              | Participant Background |

|                                                                                                                                                                                                                                                                                                                                                                                                                                                                                                                                                                                                                                                                                                                                                                                                                                                                                                                       |                                                                                                                                                                                                                                                                                                                                                                                                                                     |                                                         |
|-----------------------------------------------------------------------------------------------------------------------------------------------------------------------------------------------------------------------------------------------------------------------------------------------------------------------------------------------------------------------------------------------------------------------------------------------------------------------------------------------------------------------------------------------------------------------------------------------------------------------------------------------------------------------------------------------------------------------------------------------------------------------------------------------------------------------------------------------------------------------------------------------------------------------|-------------------------------------------------------------------------------------------------------------------------------------------------------------------------------------------------------------------------------------------------------------------------------------------------------------------------------------------------------------------------------------------------------------------------------------|---------------------------------------------------------|
| <p>a. Are you supporting other people wrt data? If so, how?</p> <p>2. How would you rate yourself in terms of data and analytics proficiency? Background?</p> <p>3. Can you give me a sense of the kinds of data that you routinely work with?</p> <p>4. What data tools do you regularly use? What for?</p> <p>5. What kinds of data do you work with?</p> <p>6. How do you get your data? Do you use multiple sources? Multiple tables or sheets in the same dataset?</p> <p>7. Do you ever inspect/eyeball/look at your raw data before and during analysis?) why? What do you need to know?</p> <p>a. If yes: "What tools do you use for this?"</p> <p>b. If no: "Why not?"</p>                                                                                                                                                                                                                                   | <p>spatial/geo, time, social network, text, KPIs etc). Probe for their experience with each kind, and their experience in combining them.</p>                                                                                                                                                                                                                                                                                       |                                                         |
| <p>Thanks for your thoughts. Let's now take a look at what you use when you are working with data. In this session, we can either walk through a past analysis you've done with these data or observe a new analysis. Given where you're at with your data, which makes more sense?</p> <p>Great! To get started, can you first give me a brief overview of your goals and major steps that you took / will take for this analysis?</p> <p>Can you briefly draw on a sheet of paper what you think the main components and relationships in the data <i>should be</i> related to what you want to find out? Draw them out like multiple tables or categories. Give these tables some names. As an example, here is a sketch of a film dataset [describe it].</p> <p>Which tables and relations are the most important?</p> <p>What aspects/ questions of these data or getting insights do you want to work with?</p> | <p><i>Moderator:</i></p> <ul style="list-style-type: none"> <li>- Show participant example sketch.</li> <li>- ask participant to sketch out their response, take a picture with their phone, and email it to us</li> <li>- Remember to record the session info to save sketch for later review.</li> </ul> <p><i>Notetakers:</i></p> <ul style="list-style-type: none"> <li>- Make a record of any participant questions</li> </ul> | <p><b>Model elicitation with participants' data</b></p> |
| <p>Thanks for this. Now I'd like you to walk me through achieving your task goals with these data, showing me which tools you use, and where you face challenges. In particular,</p> <p>Are there places where you were surprised by results? Found it challenging to get to the right result?</p> <p>Are there steps or places where the data need to be rearranged or reorganized?</p> <p>If yes – why do you do this? How?</p> <p>Are there places where you need to change, add or remove things from the data, like categories or values?</p> <p>What do you use to do this?</p> <p>Are there tasks that are difficult to do? Why?</p> <p>How do you understand how the tool goes from the raw output to the finished result? Can you explain the sequence of operations?</p>                                                                                                                                    | <p><i>Moderator:</i></p> <ul style="list-style-type: none"> <li>- Ask all probing questions, try to time this with participant actions</li> <li>- Try to ask these questions in order.</li> </ul> <p><i>Notetakers:</i></p> <ul style="list-style-type: none"> <li>- Listen for probing questions, recording responses.</li> </ul>                                                                                                  |                                                         |

|                                                                                                                                                                                                                                                                                                                  |                                                                                                                                                              |                       |
|------------------------------------------------------------------------------------------------------------------------------------------------------------------------------------------------------------------------------------------------------------------------------------------------------------------|--------------------------------------------------------------------------------------------------------------------------------------------------------------|-----------------------|
| How do you detect errors in your data?                                                                                                                                                                                                                                                                           |                                                                                                                                                              |                       |
|                                                                                                                                                                                                                                                                                                                  |                                                                                                                                                              |                       |
| <p>Thank you so much for all of your insights</p> <p>2. Is there anything that you want to comment on that I have not asked you about?</p> <p>Thanks so much for all your time today. Here's what I learned from you in our discussion:<br/><i>[Moderator to summarize a few key points. Keep it brief.]</i></p> | <p><i>Moderator:</i></p> <ul style="list-style-type: none"><li>- Ask final questions</li><li>- Summarize what you've learned from the participants</li></ul> | <p><b>Wrap up</b></p> |
